# Supplementary material for: Feedbacks, Receptor Clustering, and Receptor Restriction to Single Cells yield large Turing Spaces for Ligand-receptor based Turing Models
Source: arXiv:1407.7114 source file (2014-07-26)
Supplement: Supplementary file 1 [file Figure1_Supp.pdf]

Figure S1: Turing space of uncoupled and coupled ligand-receptor based Turing systems ($p = 0.1$ – yellow, $p = 1$ – blue, $p = 10$ – red)

| Eq. | Reaction diagram | Reaction terms | Turing space | $a_{\max}$ and the range of $b$ |
|---|---|---|---|---|
| Turing space of ligand-receptor based Turing system | | | | |
| S1 | 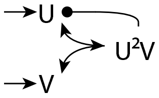  | $f = a - u + u^2 v$<br>$g = b - u^2 v$ | 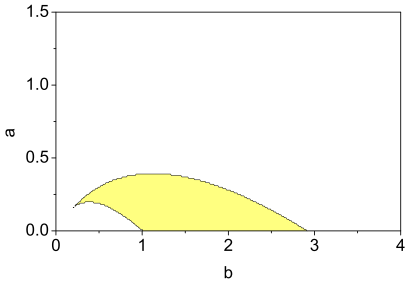  | 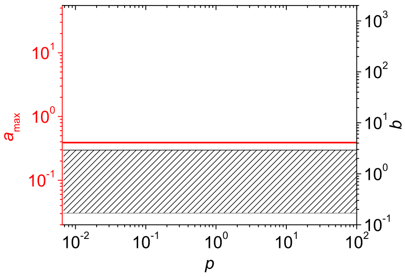  |
| Turing space of ligand-receptor based Turing systems with feedback | | | | |
| U1 | 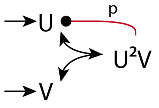  | $f = a - u + pu^2 v$<br>$g = b - u^2 v$ | 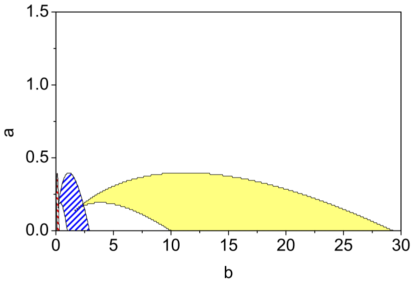  | 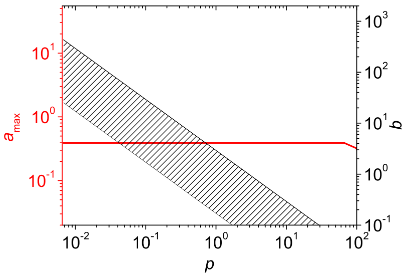  |
| U2 | 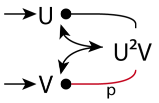  | $f = a - u + u^2 v$<br>$g = b - u^2 v + pu^2 v$ | 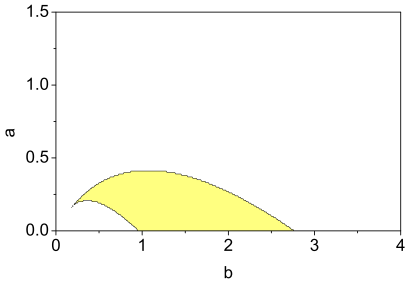  | 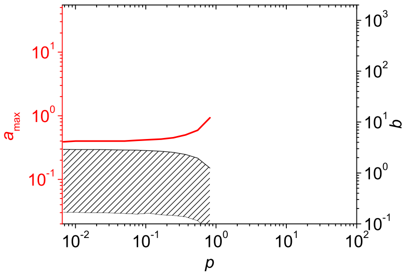  |
| U3 | 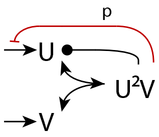  | $f = \frac{a}{1+\frac{u^2 v}{p}} - u + u^2 v$<br>$g = b - u^2 v$ | 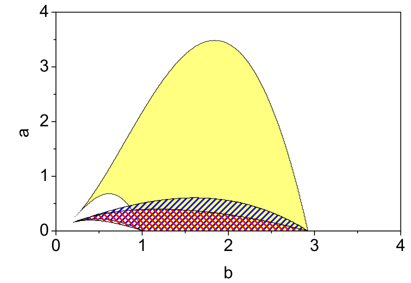  | 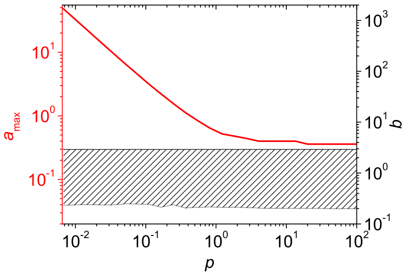  |
| U4 | 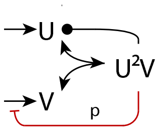  | $f = a - u + u^2 v$<br>$g = \frac{b}{1+\frac{u^2 v}{p}} - u^2 v$ | 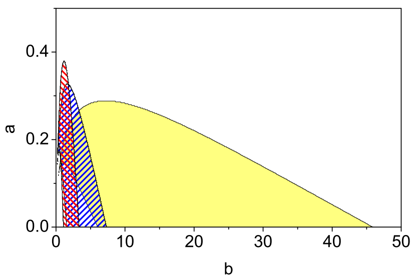  | 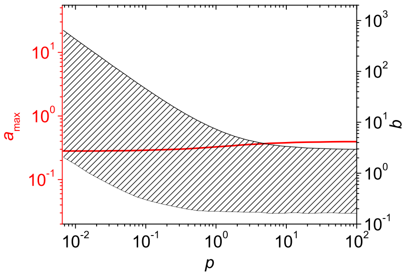  |

*continued on next page*

| Eq. | Reaction diagram | Reaction terms | Turing space | $a_{\max}$ and the range of $b$ |
|---|---|---|---|---|
| U5 | 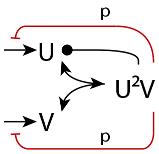 | $f = \frac{a}{1+\frac{u^2 v}{p}} - u + u^2 v$<br>$g = \frac{b}{1+\frac{u^2 v}{p}} - u^2 v$ | 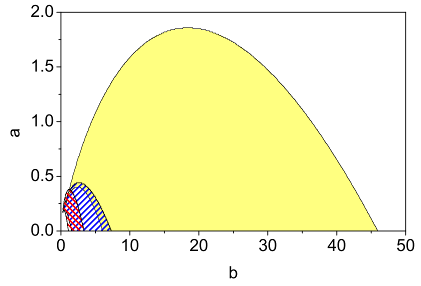 | 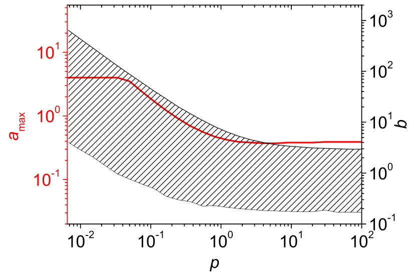 |
| U6 | 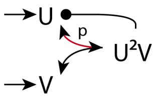 | $f = a - u + \frac{u^2 v}{p+u^2 v}$<br>$g = b - u^2 v$ | 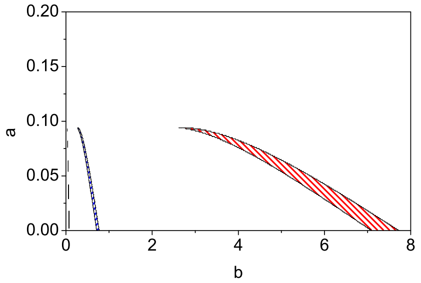 | 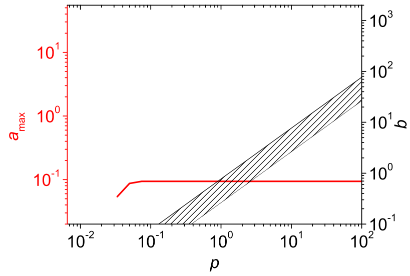 |
| U7 | 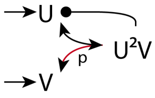 | $f = a - u + u^2 v$<br>$g = b - \frac{u^2 v}{p+u^2 v}$ | 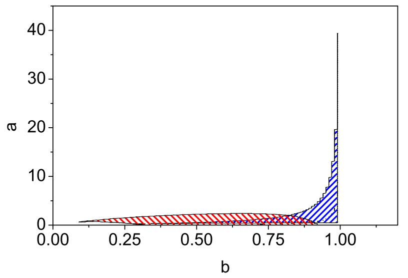 | 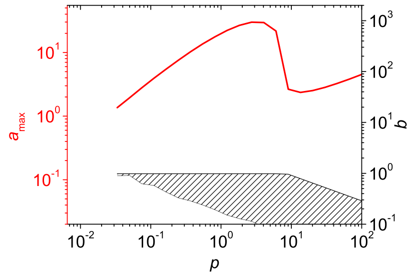 |
| U8 | 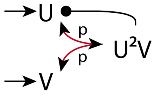 | $f = a - u + \frac{u^2 v}{p+u^2 v}$<br>$g = b - \frac{u^2 v}{p+u^2 v}$ | 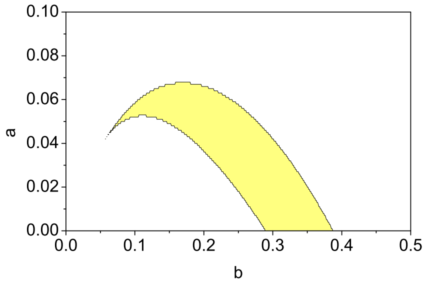 | 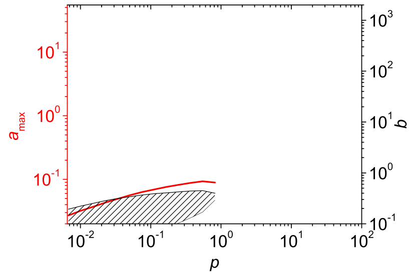 |
| U9 | 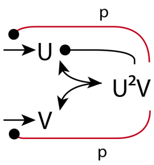 | $f = a\,\frac{u^2 v}{u^2 v+p} - u + u^2 v$<br>$g = b\,\frac{u^2 v}{u^2 v+p} - u^2 v$ | 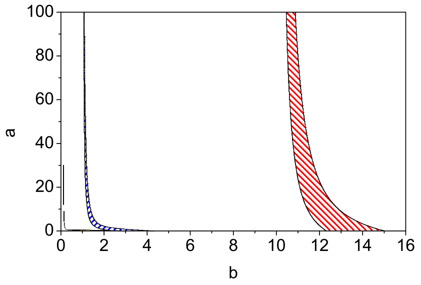 | 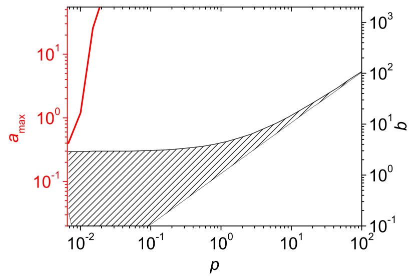 |
| U10 | 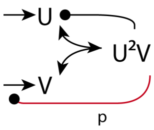 | $f = a - u + u^2 v$<br>$g = b\,\frac{u^2 v}{u^2 v+p} - u^2 v$ | 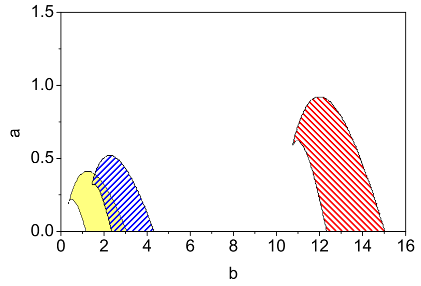 | 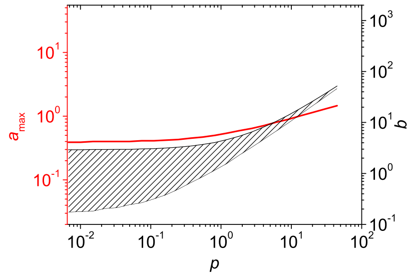 |

*continued on next page*

| Eq. | Reaction diagram | Reaction terms | Turing space | $a_{\max}$ and the range of $b$ |
|---|---|---|---|---|
| U11 | 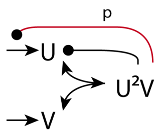 | $f = a\,\frac{u^2 v}{u^2 v + p} - u + u^2 v$<br>$g = b - u^2 v$ | 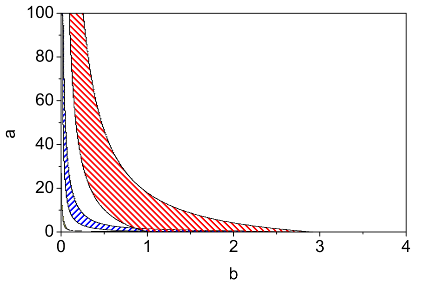 | 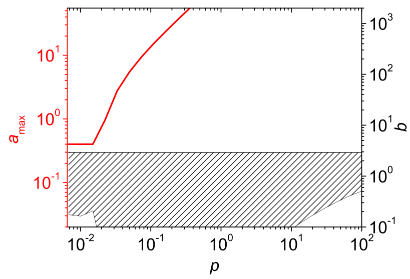 |
| Turing space of coupled ligand-receptor based Turing systems | | | | |
| C1 | 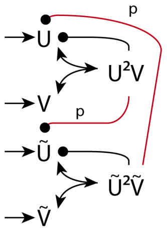 | $f = a - u + u^2 v + p\tilde{u}^2\tilde{v}$<br>$g = b - u^2 v$<br>$\tilde{f} = a - \tilde{u} + \tilde{u}^2\tilde{v} + p u^2 v$<br>$\tilde{g} = b - \tilde{u}^2\tilde{v}$ | 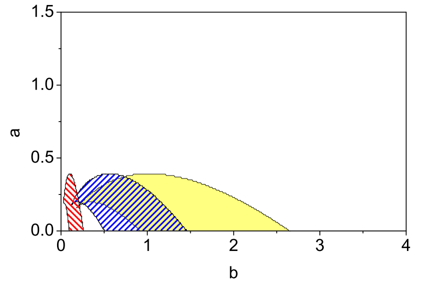 | 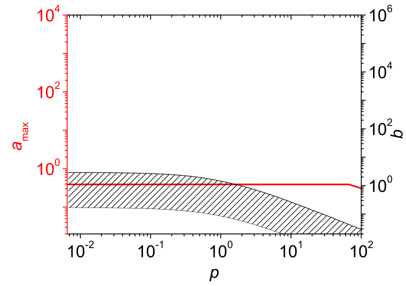 |
| C2 | 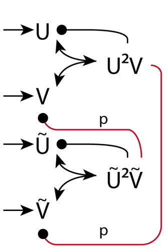 | $f = a - u + u^2 v$<br>$g = b - u^2 v + p\tilde{u}^2\tilde{v}$<br>$\tilde{f} = a - \tilde{u} + \tilde{u}^2\tilde{v}$<br>$\tilde{g} = b - \tilde{u}^2\tilde{v} + p u^2 v$ | 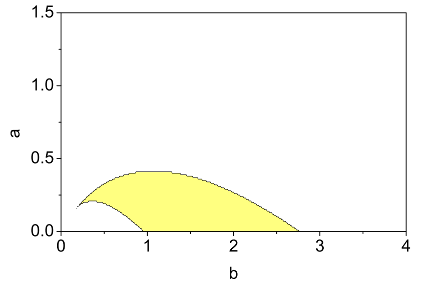 | 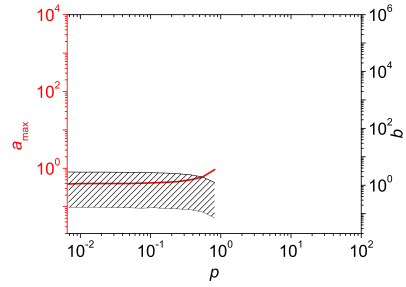 |
| C3 | 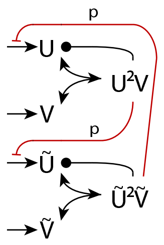 | $f = \frac{a}{1+\frac{\tilde{u}^2\tilde{v}}{p}} - u + u^2 v$<br>$g = b - u^2 v$<br>$\tilde{f} = \frac{a}{1+\frac{\tilde{u}^2\tilde{v}}{p}} - \tilde{u} + \tilde{u}^2\tilde{v}$<br>$\tilde{g} = b - \tilde{u}^2\tilde{v}$ | 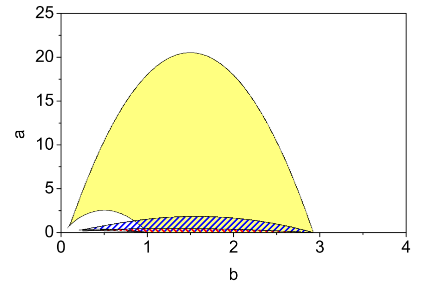 | 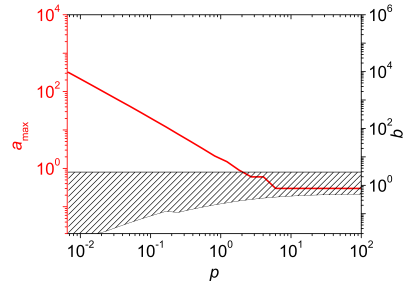 |
| C4 | 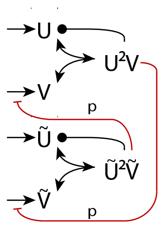 | $f = a - u + u^2 v$<br>$g = \frac{b}{1+\frac{\tilde{u}^2\tilde{v}}{p}} - u^2 v$<br>$\tilde{f} = a - \tilde{u} + \tilde{u}^2\tilde{v}$<br>$\tilde{g} = \frac{b}{1+\frac{u^2 v}{p}} - \tilde{u}^2\tilde{v}$ | 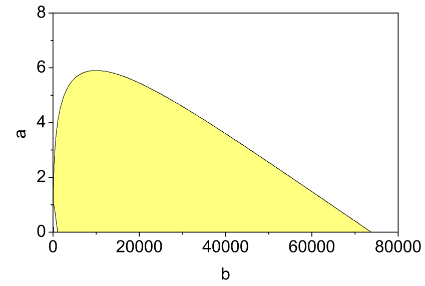 | 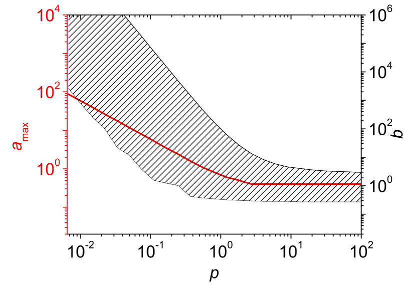 |
| C5 | 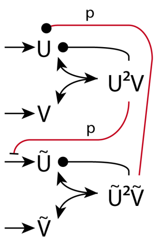 | $f = a - u + u^2 v + p\tilde{u}^2\tilde{v}$<br>$g = b - u^2 v$<br>$\tilde{f} = \frac{a}{1+\frac{u^2 v}{p}} - \tilde{u} + \tilde{u}^2\tilde{v}$<br>$\tilde{g} = b - \tilde{u}^2\tilde{v}$ | 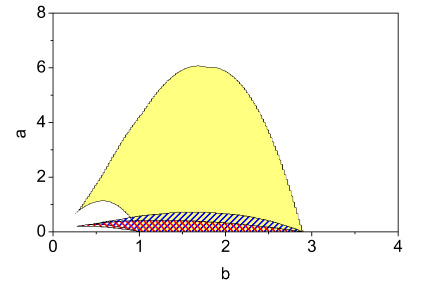 | 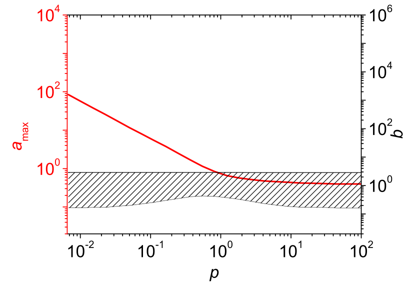 |

*continued on next page*

| Eq. | Reaction diagram | Reaction terms | Turing space | $a_{\max}$ and the range of $b$ |
|---|---|---|---|---|
| C6 | 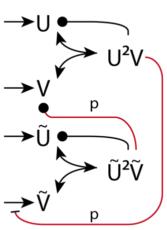 | $f = a - u + u^2 v$<br>$g = b - u^2 v + p\tilde{u}^2\tilde{v}$<br>$\tilde{f} = a - \tilde{u} + \tilde{u}^2\tilde{v}$<br>$\tilde{g} = \frac{b}{1+\frac{u^2 v}{p}} - \tilde{u}^2\tilde{v}$ | 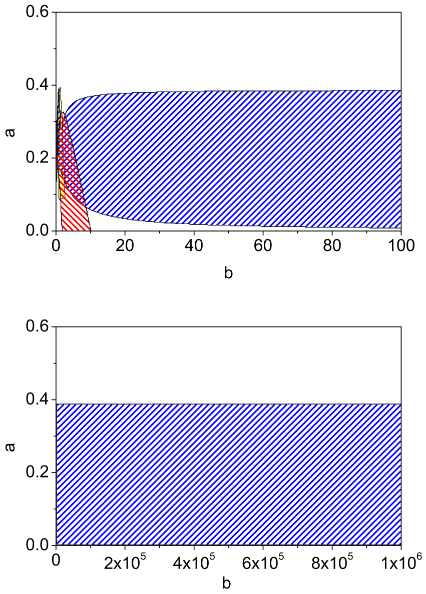 | 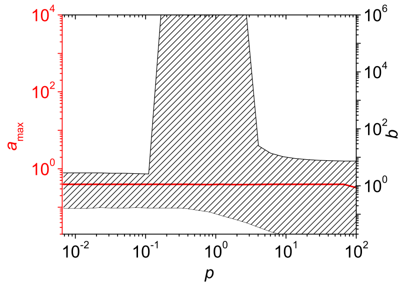 |
| C7 | 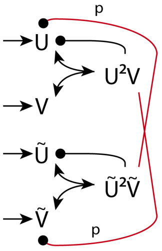 | $f = a - u + u^2 v + p\tilde{u}^2\tilde{v}$<br>$g = b - u^2 v$<br>$\tilde{f} = a - \tilde{u} + \tilde{u}^2\tilde{v}$<br>$\tilde{g} = b - \tilde{u}^2\tilde{v} + pu^2 v$ | 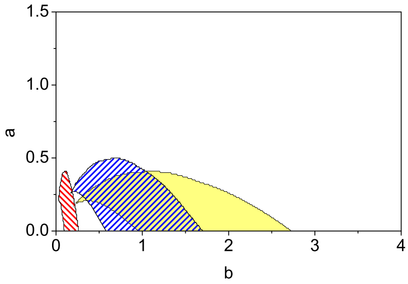 | 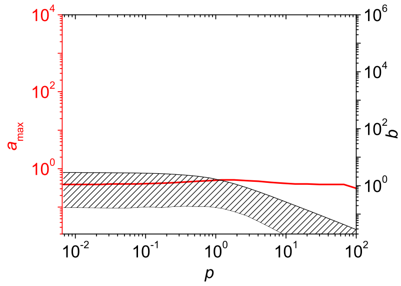 |
| C8 | 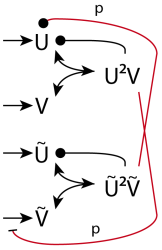 | $f = a - u + u^2 v + p\tilde{u}^2\tilde{v}$<br>$g = b - u^2 v$<br>$\tilde{f} = a - \tilde{u} + \tilde{u}^2\tilde{v}$<br>$\tilde{g} = \frac{b}{1+\frac{u^2 v}{p}} - \tilde{u}^2\tilde{v}$ | 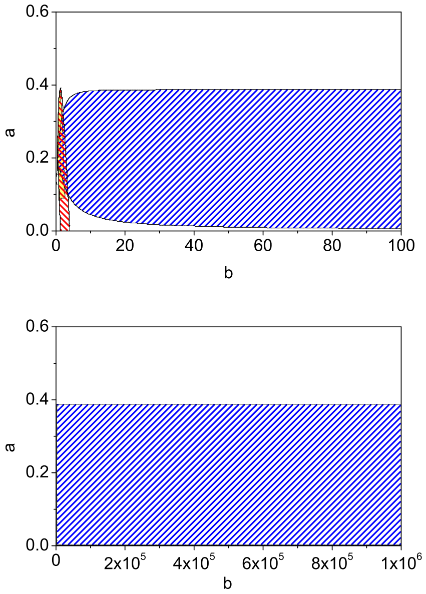 | 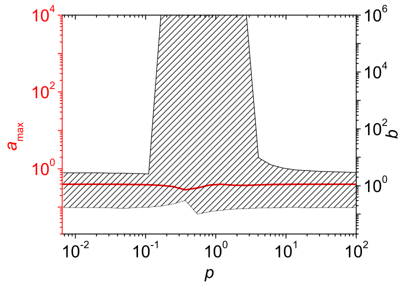 |
| C9 | 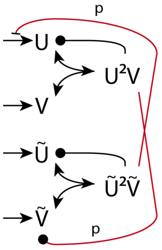 | $f = \frac{a}{1+\frac{\tilde{u}^2\tilde{v}}{p}} - u + u^2 v$<br>$g = b - u^2 v$<br>$\tilde{f} = a - \tilde{u} + \tilde{u}^2\tilde{v}$<br>$\tilde{g} = b - \tilde{u}^2\tilde{v} + pu^2 v$ | 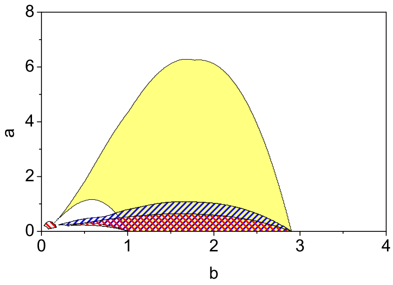 | 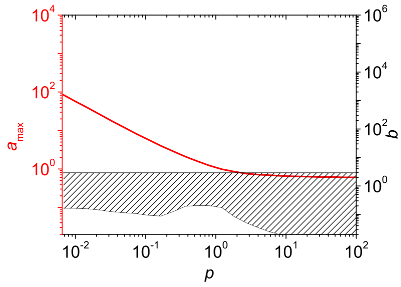 |

*continued on next page*

| Eq. | Reaction diagram | Reaction terms | Turing space | $a_{\max}$ and the range of $b$ |
|---|---|---|---|---|
| C10 | 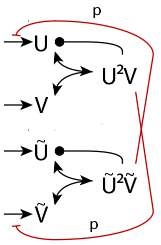 | $f=\frac{a}{1+\frac{\tilde{u}^2\tilde{v}}{p}}-u+u^2v$<br>$g=b-u^2v$<br>$\tilde{f}=a-\tilde{u}+\tilde{u}^2\tilde{v}$<br>$\tilde{g}=\frac{b}{1+\frac{u^2v}{p}}-\tilde{u}^2\tilde{v}$ | 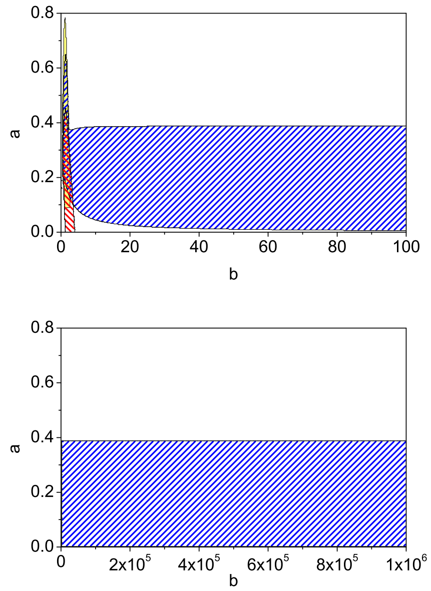 | 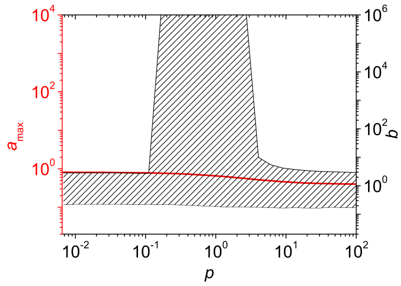 |
| C11 | 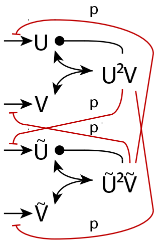 | $f=\frac{a}{1+\frac{\tilde{u}^2\tilde{v}}{p}}-u+u^2v$<br>$g=\frac{b}{1+\frac{\tilde{u}^2\tilde{v}}{p}}-u^2v$<br>$\tilde{f}=\frac{a}{1+\frac{u^2v}{p}}-\tilde{u}+\tilde{u}^2\tilde{v}$<br>$\tilde{g}=\frac{b}{1+\frac{u^2v}{p}}-\tilde{u}^2\tilde{v}$ | 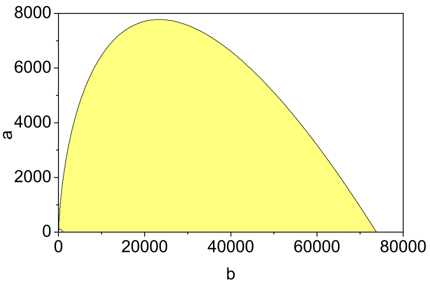 | 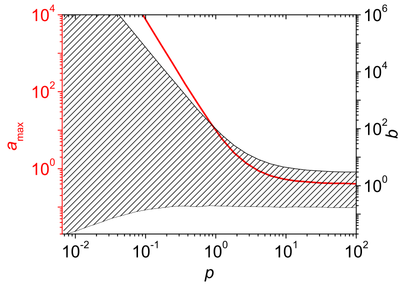 |
| C12 | 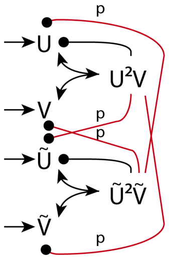 | $f=a-u+u^2v+p\tilde{u}^2\tilde{v}$<br>$g=b-u^2v+p\tilde{u}^2\tilde{v}$<br>$\tilde{f}=a-\tilde{u}+\tilde{u}^2\tilde{v}+pu^2v$<br>$\tilde{g}=b-\tilde{u}^2\tilde{v}+pu^2v$ | 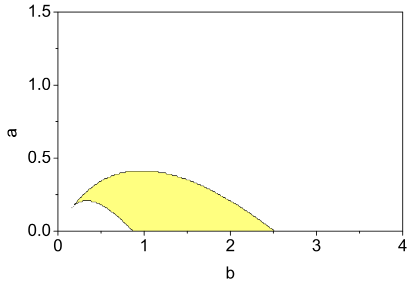 | 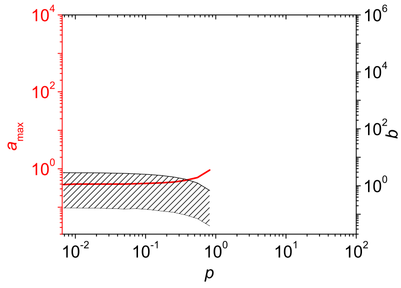 |
